# Supplementary material for: Lighter, Better, Faster Multi-Source Domain Adaptation with Gaussian Mixture Models and Optimal Transport
Source: arXiv:2404.10261 source file (2024-08-21)
Supplement: Supplementary file 1 [file 6_supplementary.tex]

\section{Introduction}

In this supplementary materials, we provide additional details about our theoretical and experimental results.

\section{Proofs}

\subsection{Proof for Theorem 1}

\begin{theorem}\label{thm:appx_first_order_mw2}
    Let $P$ and $Q$ be two \glspl{gmm} with components $P_{i} = \mathcal{N}(\mathbf{m}_{i}^{(P)}, (\mathbf{s}_{i}^{(P)})^{2})$ (resp. $Q_{j}$) and $\omega^{\star}$ be the solution of eq. 10. The first-order optimality conditions of $\mathcal{MW}_{2}^{2}$, with respect $\mathbf{m}_{i}$ and $\mathbf{s}_{i}$ are given by,
    \begin{align}
        \mathbf{m}_{i} = T_{\omega}(\mathbf{m}_{i}^{(P)}) = \sum_{j=1}^{K_{Q}}\dfrac{\omega_{ij}^{\star}}{p_{i}}\mathbf{m}_{j}^{(Q)}\text{, and }
        \mathbf{s}_{i} = T_{\omega}(\mathbf{s}_{i}^{(P)}) = \sum_{j=1}^{K_{Q}}\dfrac{\omega_{ij}^{\star}}{p_{i}}\mathbf{s}_{j}^{(Q)}.\label{eq:appx_first_order_mw}
    \end{align}
\end{theorem}

\begin{proof}
    Under the \gls{gmm}-\gls{ot} framework, the $2-$mixture Wasserstein distance is given by,
    \begin{align*}
        \mathcal{MW}_{2}(P, Q)^{2} = \sum_{i=1}^{K_{P}}\sum_{j=1}^{K_{Q}}\omega_{ij}^{\star}\mathcal{W}_{2}(P_{i},Q_{j})^{2},
    \end{align*}
    where $\omega_{ij}^{\star}$ is the mass transported from component $i$ in $P$ to component $j$ in $Q$ by the solution to the \gls{gmm}-\gls{ot} problem. Since $P_{i}$ and $Q_{j}$ are axis-aligned Gaussian measures,
    \begin{align*}
        \mathcal{W}_{2}(P_{i}, Q_{j})^{2} = \lVert \mathbf{m}_{i} - \mathbf{m}_{j}^{(Q)}\rVert_{2}^{2} + \lVert \mathbf{s}_{i} - \mathbf{s}_{j}^{(Q)}\rVert_{2}^{2},
    \end{align*}
    where $\mathbf{m}_{i}$ and $\mathbf{s}_{i}$ are the free parameters we want to determine. Henceforth we derive the first-order conditions for $\mathbf{m}_{i}$. The derivations for $\mathbf{s}_{i}$ are completely analogous. By linearity,
    \begin{align*}
        \dfrac{\partial \mathcal{MW}_{2}^{2}}{\partial \mathbf{m}_{i}} = 2\sum_{j=1}^{K_{Q}}\omega_{ij}^{\star}(\mathbf{m}_{i}-\mathbf{m}_{j}^{(Q)}) = 2\biggr{(}p_{i}\mathbf{m}_{i} - \sum_{j=1}^{K_{Q}}\omega_{ij}^{\star}\mathbf{m}_{j}^{(Q)}\biggr{)},
    \end{align*}
    equating this last term to $0$, one gets the desired equality.
\end{proof}

The result of theorem~\ref{thm:appx_first_order_mw2} is quite similar to the barycentric mapping of~\cite{courty2014domain,courty2016optimal} which was previously used to map points in $P$ to points in $Q$. Here, we transport the parameters of \glspl{gmm} instead.

\subsection{Proof of Theorem 2}

\begin{theorem}\label{thm:appx_first_order_smw2}
    Under the same conditions of theorem~\ref{thm:appx_first_order_mw2}, let $P_{i}$ and $Q_{j}$ be equipped with labels $\mathbf{v}_{i}^{(P)}$ and $\mathbf{v}_{j}^{(Q)}$. The first order optimality conditions of $\mathcal{SMW}_{2}$ with respect $\mathbf{m}_{i}$ and $\mathbf{s}_{i}$ are given by eq.~\ref{eq:appx_first_order_mw}. Furthermore, for $\mathbf{v}_{i}$,
    \begin{align}
        \mathbf{v}_{i} = T_{\omega}(\mathbf{v}_{i}^{(P)}) = \sum_{j=1}^{K_{Q}}\dfrac{\omega_{ij}^{\star}}{p_{i}}\mathbf{v}_{j}^{(Q)}.\label{eq:appx_first_order_smw}
    \end{align}
\end{theorem}

\begin{proof}
    Note that the label distance term added to $\mathcal{SMW}$ does not interfere with the terms on $\mathbf{m}_{i}$ and $\mathbf{s}_{i}$, hence the optimality conditions with respect these variables remain unchanged. Due the independence of these terms, the first-order optimality condition with respect $\mathbf{v}_{i}$ is,
    \begin{align*}
        \dfrac{\partial \mathcal{SMW}_{2}^{2}}{\partial \mathbf{v}_{i}} = 2\beta\sum_{j=1}^{K_{Q}}\omega_{ij}^{\star}(\mathbf{v}_{i}-\mathbf{v}_{j}^{(Q)}) = 2\beta\biggr{(}p_{i}\mathbf{v}_{i} - \sum_{j=1}^{K_{Q}}\omega_{ij}^{\star}\mathbf{v}_{j}^{(Q)}\biggr{)},
    \end{align*}
    which, for $\beta > 0$, is zero if and only if $\mathbf{v}_{i} = T_{\omega}(\mathbf{v}_{i}^{(P)})$.
\end{proof}

\subsection{Derivation of Algorithm 1}

In this section, we derive the first-order conditions for the functional $B \mapsto \sum_{c}\lambda_{c}\mathcal{SMW}_{2}(B, P_{c})^{2}$. Let $B$ be parametrized by $\theta_{B} = \{(\mathbf{m}_{i}^{(B)}, \mathbf{s}_{i}^{(B)},\mathbf{v}_{i}^{(B)})\}_{i=1}^{K_{B}}$, where these variables are initialized randomly as in algorithm 1. For fixed $\theta_{B}$, we find $\omega_{1}^{\star},\cdots,\omega_{C}^{\star}$ transport plans. Then, for fixed transport plans, we solve,
\begin{align*}
    \argmin{\theta_{B}}\mathcal{L}(\theta_{B}) &= \sum_{c=1}^{C}\lambda_{c}\sum_{i=1}^{K_{B}}\sum_{j=1}^{K_{P}}\omega_{c,i,j}^{(\star)}M_{c,i,j},\\
    \text{where }M_{c,i,j} &= \lVert \mathbf{m}_{i}^{(B)} - \mathbf{m}_{j}^{(P_{c})}\rVert_{2}^{2} + \lVert \mathbf{s}_{i}^{(B)} - \mathbf{s}_{j}^{(P_{c})}\rVert_{2}^{2} + \beta\lVert \mathbf{v}_{i}^{(B)} - \mathbf{v}_{j}^{(P_{c})}\rVert_{2}^{2}
\end{align*}
which can be optimized by taking derivatives with respect $\mathbf{m}^{(B)}_{i}$, $\mathbf{s}^{(B)}_{i}$ and $\mathbf{v}^{(B)}_{i}$. For instance, taking the derivative of $\mathcal{L}(\theta_{B})$ with respect $\mathbf{m}_{i}^{(B)}$,
\begin{align*}
    \dfrac{\partial \mathcal{L}}{\partial\mathbf{m}_{i}^{(B)}} = 2\sum_{c=1}^{C}\lambda_{k}\sum_{j=1}^{K_{P}}\omega_{c,i,j}^{\star}(\mathbf{m}_{i}^{(B)} - \mathbf{m}_{j}^{(P_{c})}) = \dfrac{2}{K_{B}}\mathbf{m}_{i}^{(B)} - 2\sum_{c=1}^{C}\lambda_{c}\sum_{j=1}^{K_{P}}\omega_{c,i,j}^{\star}\mathbf{m}_{j}^{(P_{c})}
\end{align*}
setting the derivative to $0$, one has,
\begin{align*}
    \mathbf{m}_{i}^{(B)} &= \sum_{c=1}^{C}\lambda_{c}T_{\omega_{c}^{\star}}(\mathbf{m}_{i}^{(B)}).
\end{align*}
Similar results can be acquired for $\mathbf{s}_{i}^{(B)}$ and $\mathbf{v}_{i}^{(B)}$ by taking the appropriate derivatives.

\section{Additional Experiments}

\begin{wrapfigure}{r}{0.5\textwidth}
    \centering
    \includegraphics[width=0.7\linewidth]{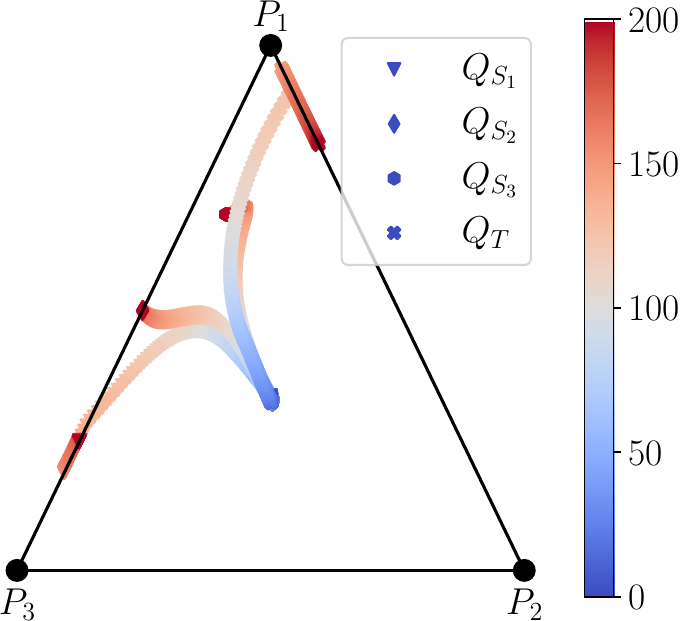}
    \caption{Evolution of barycentric coordinates over the simplex $\Delta_{C}$.}
    \label{fig:simplex_spread}
    \vspace{-0.75cm}
\end{wrapfigure}
\textbf{Toy Example.} We analyze the evolution of the atoms in \gls{gmm}-\gls{dadil} as training progresses (figure~\ref{fig:atom-evolution}). Note that, initially, the means are close to each other, so there are no distinction between classes. Likewise, in our initialization, the labels are uniform histograms over the classes, so that the atoms are \emph{not certain} about which class they represent. With 50 iterations, \gls{dadil} manages to spread the class clusters, but, at this point, the barycentric coordinates of each domain are still too similar (i.e., $\lambda_{\ell} \approx \mathds{1}_{K} / K$, see figure 2.a in the main paper). As the training progresses, the barycentric coordinates of the different domains begins to spread over the simplex $\Delta_{C}$ (see figure~\ref{fig:simplex_spread}). As a result, the atoms begin to be different from each other (compare figures~\ref{fig:atom-evolution} (b) and (c)).

\noindent\textbf{Hyper-parameter Setting:} Here we detail the hyper-parameter setting for our method. \gls{gmm}-\gls{wbt} involves a single hyper-parameter: the number of components $K$ in the \glspl{gmm}. \gls{dadil} involves a few other parameters: the number of atoms $C$, the learning rate $\eta$ and the number of optimization steps $N_{iter}$. As~\cite{montesuma2023learning}, we use Adam~\cite{kingma2013auto} for optimizing eq. 16 (see main paper). Over all our experiments we set $\eta = 10^{-1}$. We show our hyper-parameters in table~\ref{tab:hyperparam_setting}. We remark that, as we analyze in Fig 6. b (main paper), our proposed methods, especially \gls{gmm}-\gls{dadil}, are robust to the choice of hyper-parameters.

\begin{table}[ht]
    \centering
    \caption{Hyper-parameter setting}
    \begin{tabular}{lcccc}
        \toprule
        Benchmark & $K$ (GMM-WBT) & $K$ (GMM-DaDiL) & $C$ & $N_{iter}$\\
        \midrule
        Office 31 & 155 & 186 & 3 & 150 \\
        Office-Home & 910 & 455 & 4 & 150\\
        TEP & 261 & 174 & 7 & 150 \\
        CWRU & 30 & 90 & 5 & 200\\
        \bottomrule
    \end{tabular}
    \label{tab:hyperparam_setting}
\end{table}

\begin{figure}[ht]
    \centering
    \begin{subfigure}{0.75\linewidth}
        \includegraphics[width=\linewidth]{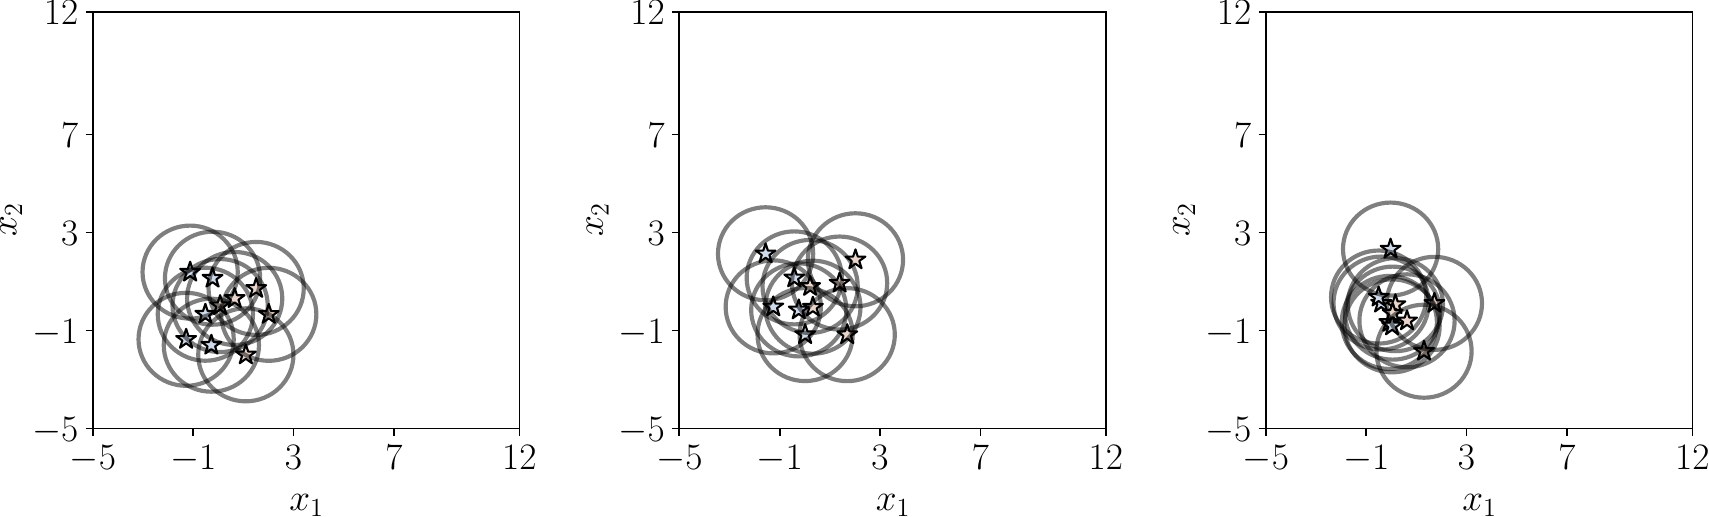}
        \caption{1st iteration.}
    \end{subfigure}
    \begin{subfigure}{0.75\linewidth}
        \includegraphics[width=\linewidth]{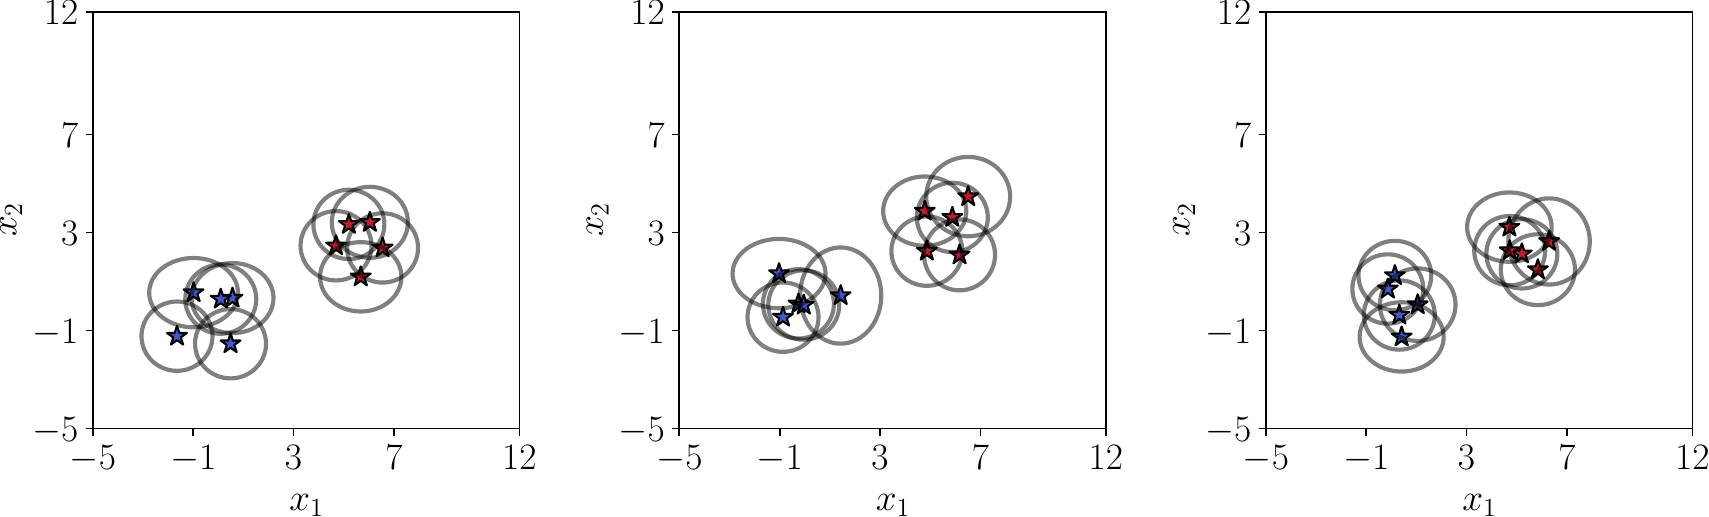}
        \caption{50th iteration.}
    \end{subfigure}
    \begin{subfigure}{0.75\linewidth}
        \includegraphics[width=\linewidth]{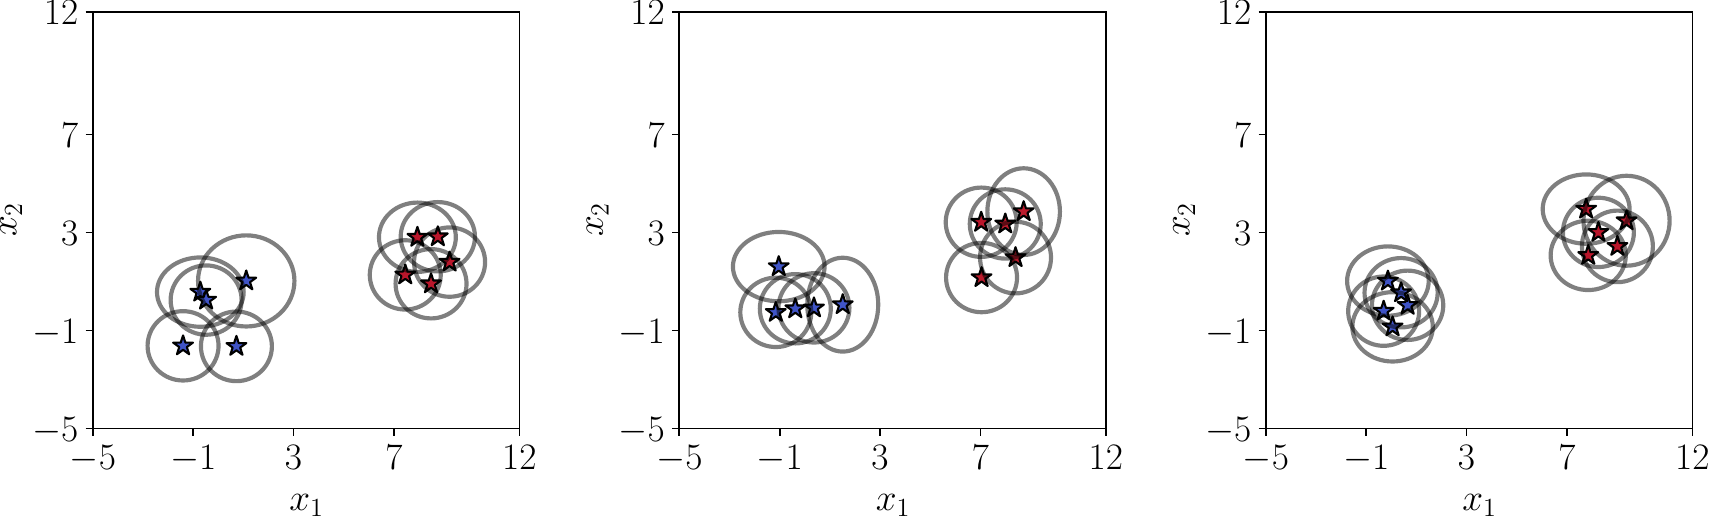}
        \caption{100th iteration.}
    \end{subfigure}
    \begin{subfigure}{0.75\linewidth}
        \includegraphics[width=\linewidth]{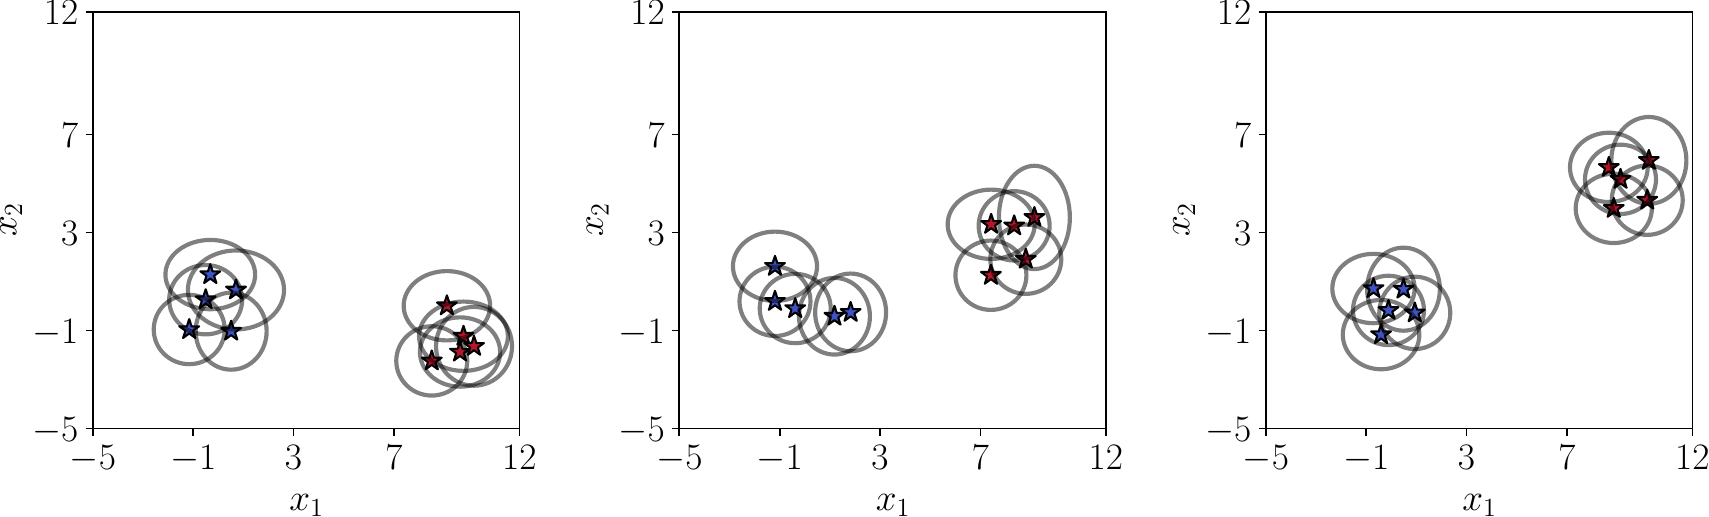}
        \caption{150th iteration.}
    \end{subfigure}
    \begin{subfigure}{0.75\linewidth}
        \includegraphics[width=\linewidth]{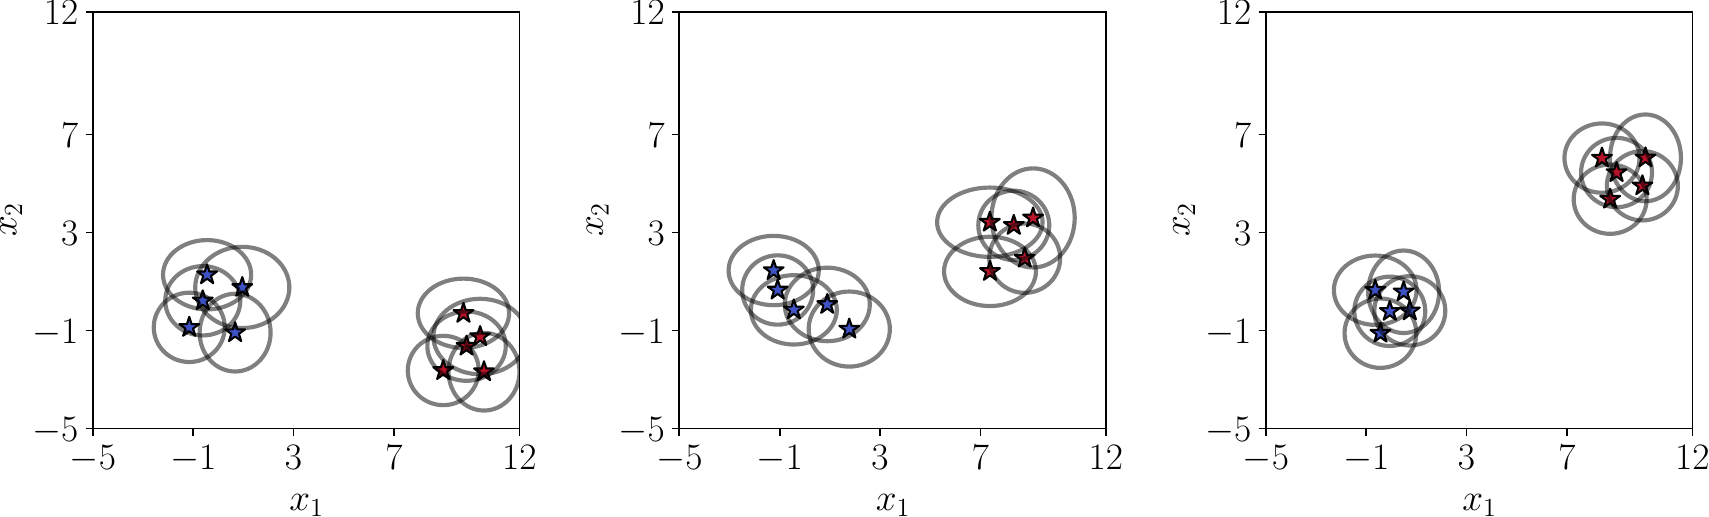}
        \caption{200th iteration.}
    \end{subfigure}
    \caption{Evolution of atoms as the training progresses.}
    \label{fig:atom-evolution}
\end{figure}
